# Supplementary material for: Nanosecond magnetization dynamics during spin Hall switching of in-plane magnetic tunnel junctions
Source: arXiv:1612.06463 ancillary file (2017-02-01)
Supplement: Supplementary file 1 [file Supplemental-Information.pdf]

# Nanosecond magnetization dynamics during spin Hall switching of in-plane magnetic tunnel junctions

G. E. Rowlands[1,†], S. V. Aradhya[1,†], S. Shi[1], E. H. Yandel[1], J. Oh[1], D. C. Ralph[1,2], R. A. Buhrman[1]

1. Cornell University, Ithaca, New York 14853, USA

2. Kavli Institute at Cornell, Ithaca, New York 14853, USA

† These authors contributed equally to this work

## Supplementary Information

## Fabrication of 3T-MTJs

Our multilayer films are deposited onto thermally oxidized high-resistivity ($\varrho$>10,000 Ωcm) Si wafers using DC and RF magnetron sputtering. The films consist of the following generalized set of layers: || SiOx | spin Hall channel | free-layer | MgO | reference-layer | capping-layer. We perform a systematic study of the effect of the dipole field and pinning of the reference layer on the switching dynamics of the free layer by implementing three types of reference layers: "thick" reference layer which has pinning provided solely by its shape anisotropy; "Pinned" reference layer which uses the exchange bias from an adjacent IrMn antiferromagnetic layer; "SAF" reference layer which reduces the stray field; "SAF+Pinned" multilayer which provides both reduced stray field and pinning by IrMn exchange bias. The detailed stack structure for each type of device presented in the manuscript is (thicknesses in nm, FeCoB = $Fe_{60}Co_{20}B_{20}$, CoFeB = $Co_{60}Fe_{20}B_{20}$, CoFe = $Co_{70}Fe_{30}$):

**Ta-(thick ref)**: || SiOx | Ta (6) | FeCoB (1.8) | MgO (1.6) | FeCoB (3.5) | Ta (4) | Ru (4)
**Pt-(thick-ref):** || SiOx | Ta (1) | Pt (5) | Hf (0.5) | FeCoB (1.6) | MgO (1.6) | FeCoB (4) | Hf (3) | Ru (4)
**Pt-(pinned ref)**: || SiOx | Ta (1) | Pt (5) | Hf (0.5) | FeCoB (1.6) | MgO (1.6) | FeCoB (2.4) | IrMn (10) | Hf (1) | Ru (4)
**Pt-SAF:** || SiOx | Ta (1) | Pt (5) | Hf (0.5) | FeCoB (1.6) | MgO (1.6) | FeCoB (2.4) | Ru (1) | FeCoB (2.6) | Hf (3) | Ru (4)
**Pt-(SAF+pinning)** (both strongly and weakly pinned): || SiOx | Ta (1) | Pt (5) | Hf (0.7) | FeCoB (1.4) | MgO (~1.6) | CoFeB | Ta | CoFeB | CoFe | Ru | CoFe | IrMn | Ru (4)

For the case of the Pt channel, the purpose of the 1 nm Ta underlayer was to promote a smoother film, and to provide improved control over the magnetic anisotropy of the free layer of the MTJ; the Pt is sufficiently thick relative to its spin diffusion length (~2 nm)[1] that the Ta does not contribute any significant spin Hall torque on the MTJ. The purpose of the Hf insertion layer in the Pt devices is to minimize intermixing at the Pt/FeCoB interface, to reduce the magnetic damping and to improve spin-Hall torque efficiency $\xi_{SH}$, following Nguyen *et al.*[2] The amorphous Hf layer by itself produces negligible spin-orbit torque.[3]

Using Deep-UV photolithography and $Ar^+$ ion milling, the stacks are patterned into 335 nm wide, 600 nm long channels. Using an aligned electron beam lithography exposure, we define elliptical

MTJs of 60×210 $nm^2$ lateral extent in the center of the channels. The pillars are patterned by ion milling, and the etch process is terminated when traces of the channel material become visible in the etch chamber's endpoint detector. An SEM micrograph of a device at this stage (with photoresist) is shown in Fig. 1(b). After protecting the devices with evaporated $SiO_2$, electrical connections are established to the channel and top contact of the MTJ by means of a liftoff process. The devices are annealed at 300 C for 30 minutes in a vacuum of $8\times10^{-7}$ Torr, during which time the "pinned-ref" and "SAF + weak pinning" devices are subject to a 1.5 kG field along their long axes, while the "SAF + strong pinning" devices are instead subject to a 5.0 kG field. Thereafter, the thick-reference-layer devices possess a TMR ≈ 80% and an RA ≈ 400 $\Omega\mu m^2$, while the pinned and SAF devices suffer from reduced TMRs of 20% and 30%, respectively. The residual dipole fields ($H_{dip}$) are shown in Table 1 of the main text. The reference layers in the "pinned-ref" devices are characterized by an exchange bias field $H_{ex}$ = 250 G and coercive field $H_c$ ≥ 100 G. The "SAF + weak pinning" and "SAF + strong pinning" devices were fabricated with optimized materials stacks from Canon Anelva Corp., and they have a TMR ≈ 100% and RA ≈ 250 $\Omega\mu m^2$. The $H_{ex}$ in the "SAF + strong pinning" devices is ~2500 G. Further optimization of these reference layer structures will obviate the need for external fields during operation.

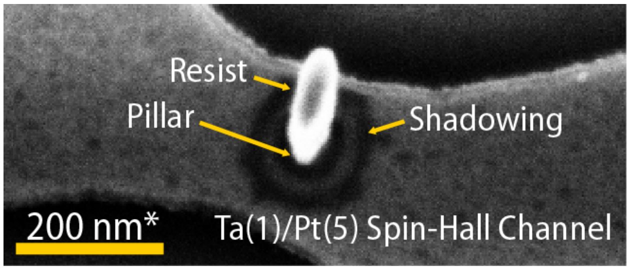


Figure S1: Tilted SEM micrograph of the pillar after milling but prior to oxide protection and liftoff. Scale is approximate due to sample tilt.

# Pulse switching measurement

The resistance of the MTJ (across the top lead and one half of the bottom channel) is measured by a lock-in amplifier connected across a voltage divider formed by the MTJ and a 10 MΩ reference resistor. For measurements of our devices' fast pulse response we employ two Picosecond Pulse Labs 10,070A pulse generators routed through a voltage combiner, the capacitive port of a bias-tee, and finally through microwave probes to the device leads (Fig. S2). One of the pulse generators is used to apply rectangular switching pulses of varying amplitude $V$ and duration, while the other is used to apply shallow reset pulses at the 10 ns maximum pulse duration $\tau$ (both pulses have 65 ps rise time and 100 ps fall time). Pulses delivered to the write channels are partially reflected given the impedance mismatch from our transmission lines, so we calculate[4] the current densities delivered to the channel

$$J = V_{corr}(1+\Gamma) / R_w A \tag{1}$$

in terms of the channel cross-sectional area $A$, the reflection coefficient $\Gamma = (R_w - 50\ \Omega)/(R_w + 50\ \Omega)$, and the pulse voltage $V_{corr}$ that corrects $V$ for losses in the circuit external to the device. For Ta|Pt|Hf channels the total write path resistance $R_w$ is typically 0.5–1.5 kΩ, depending on the amount of over-etching during the pillar definition process. Our Ta devices have higher $R_w$ = 3.5 kΩ consistent with the higher Ta resistivity. These $R_w$ values include a 5□ contribution from

current spreading in our extended lead geometry in addition to the 2□ contribution from the actual channel. Thus, in integrated devices lacking expansive leads, one expects to achieve write impedances closer to 200-300 Ω for Ta|Pt|Hf channels, substantially lower than can realistically be obtained in two-terminal MTJs of the same size.

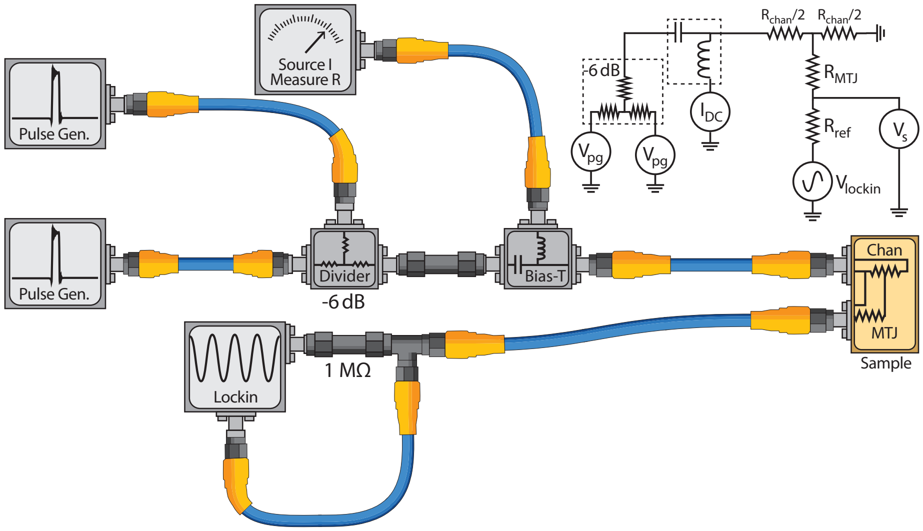


Figure S2: Pulse switching measurement setup. The inset shows the equivalent circuit: we measure the device resistance in a voltage divider with a 1 MΩ reference resistor.

# Simulations of Magnetostatics

For devices with a thick FeCoB(4) reference layer, the prominent curvature of the P state resistance shown in Fig. S3(a) suggests the development of a micromagnetic state in either or both of the magnetic layers. Accordingly, we simulated[5] the $T = 0$ K micromagnetic reversal curves for our devices. For the free layer, we used values of the saturation magnetization $M_s = 1550\times10^3$ A/m and perpendicular anisotropy field $H_k = 9700$ Oe obtained in nearly identical devices in Nguyen *et al.* (2015).[2] The reference layer was assumed to posess the same $M_s$ but no perpendicular anisotropy. We assumed an exchange constant $A = 2\times10^{-11}$ J/m$^3$ and a (1.5 nm)$^3$ cubic spatial discretization. All layer thicknesses were rounded to the nearest multiple of 1.5 nm. The hysteresis curves were calculated for devices with a perfectly elliptical 60×180 nm$^2$ cross-section (within the constraints of the cell size), as well as for devices with a rough edge profile computed directly from SEM images of our devices.

In devices with a smooth elliptical profile, the simulations produced abrupt AP→P and P→AP transitions consistent with a Stoner-Wohlfarth reversal, as seen in Fig. S3(b). The introduction of pinning sites along the edges allowed the magnetization to gradually bend away from the uniform state. In the P state the magnetizations scissor away from one another in order to reduce their mutual dipole energy, as seen in Fig. 1(d). In the AP state, however, the stray fields from either layer saturated the other layer such that this curvature was minimized as seen in Fig. 1(e). Accordingly, a sharp AP→P transition was still observed while the opposite transition maintains a substantial curvature. This behavior resulted in an asymmetric hysteresis loop, also shown in Fig.

S3(b), consistent with that observed in experiments. As mentioned in the main text, the use of a pinned and SAF reference layer stacks results in a reduced stray field (either by virtue of reduced thickness or intentional field cancellation). Thus, relatively square hysteresis loops are restored, such as that seen for an SAF reference layer in Fig. 1(c). In these systems, as the curvature is reduced the micromagnetic behavior becomes less important.

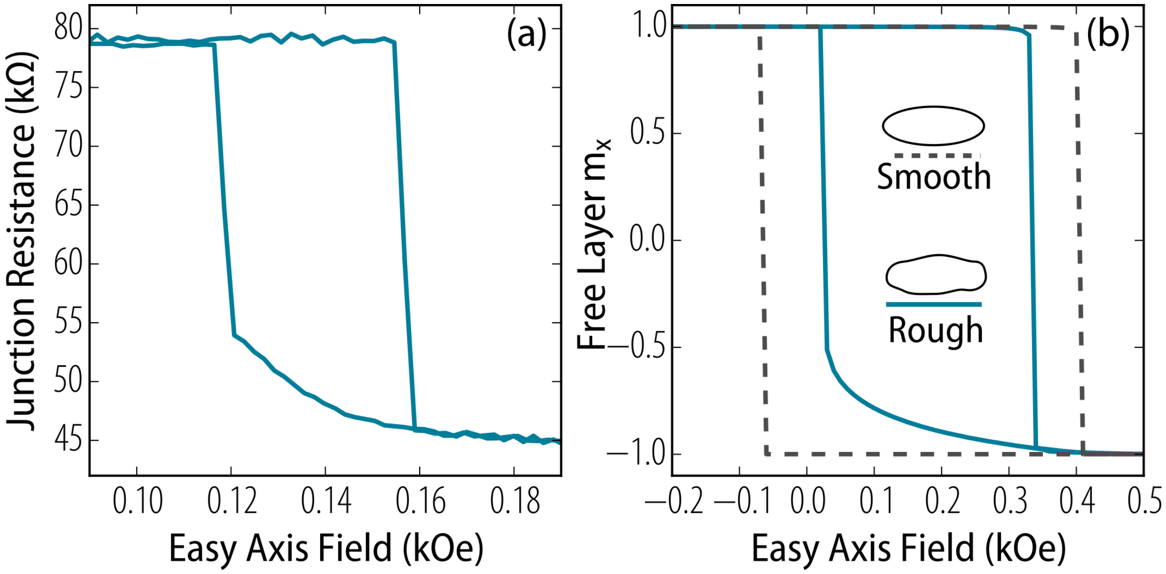


Figure S3: (a) Measured hysteresis loop of a sample with a thick FeCoB(4) reference layer. (b) Simulated hysteresis loops for the free layer/reference layer system with a smooth (dotted lines) and rough (solid blue lines) edge profile.

## Simulations of Switching Dynamics

Given the sin $\theta$ angular dependence of spin torque and the notable micromagnetic curvature observed in simulations of magnetostatic reversal, we surmise that micromagnetics will play an important role in the nature of fast reversal by the SHE. As such, we perform simulations of spin-torque induced magnetization reversal using the same parameters mentioned above (including the rough edge profile), assuming a spin Hall effect strength $\xi_{SH}$=+0.08 similar to that observed in our samples, and taking a damping value $\alpha$ = 0.016 measured on continuous films using flip-chip FMR. Furthermore, we assume that there is no field-like component of the spin torque from the SHE. As detailed in the main text, the inclusion of the as-of-yet neglected Oersted field from the SHE channel allows us to identify the source of switching timescale asymmetry. We assume a uniform magnetic field $\boldsymbol{H}_{\mathrm{Oe}} = -\mu_0 J t\, \hat{x}/2$ calculated from the current density $J$ and channel thickness $t$. We evolve the same micromagnetic system starting from stable configurations at the center of the calculated hysteresis loops (220 Oe). The simulated current pulses (which are inputs to both the Oersted field and SHE) are given linear rising and falling slopes of 65 and 100 ps, respectively, in approximate accordance with the pulse shapes used in the experimental system.

The data in Figs. 3(a-f) of the main text are the results of simulations using a reference layer thickness of 3.0 nm. This thickness is reduced to 1.5 nm for Figs. 3(g,h), which reduces the

required offset field to around 120 Oe. A pinning field of 2 kOe (corresponding to the measured pinning strength of our "strongly pinned" devices) is applied to the reference layer only.

Each phase diagram is calculated using an adaptive refinement method to identify the fine structure of the switching phase boundary — a rectilinear scan of this phase space could easily miss such complexity.

Spur-like features evident in many of the phase diagrams of Fig. 3 can also be observed in macrospin simulations and are caused by the magnetization passing close to the hard-axis energy saddle point. Magnetization precession slows near the saddle point (and more generally near the separatrix dividing in- and out-of-plane orbits), leading to failed switching attempts and interesting features in the phase diagrams. Switching phase diagrams from macrospin simulations of an isolated magnetic free layer are shown in Fig. S4 for comparison. As seen in Fig. S4(b), these spurs are eliminated when macrospin simulation are performed at $T$ = 4 K. We did not calculate finite temperature micromagnetic phase diagrams given the formidable computational burden for doing so, but they should resemble blurred versions of the diagrams seen in Fig. 3.

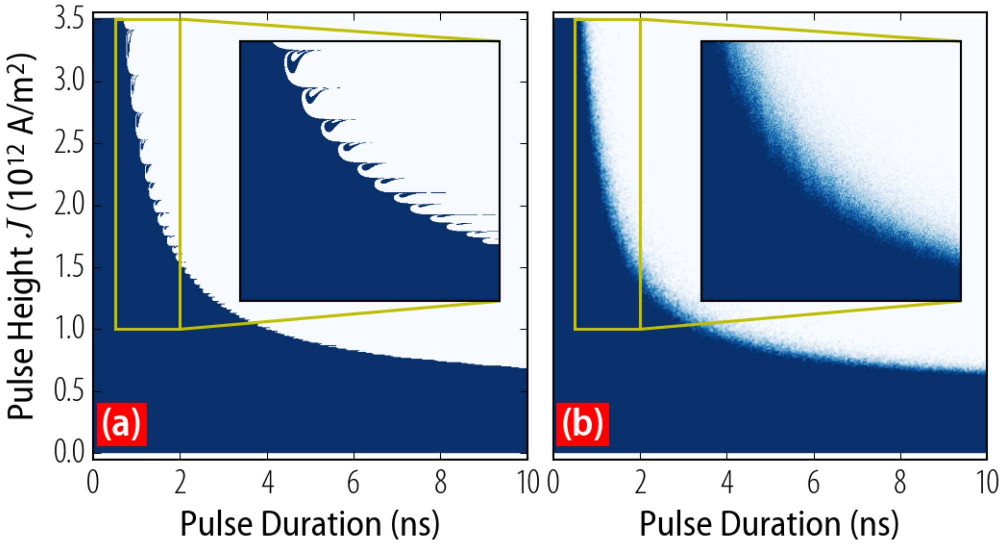


Figure S4: (a) Simulation of $T$ = 0 K macrospin dynamics showing similar spurs as in the micromagnetic simulations. (b) Simulations at $T$ = 4 K show that these features are washed out by small thermal energy scales.

While the phase diagrams of Figure 3 in the main text provide an overview of the complex switching behavior in this system, we show in Fig. S5 some example trajectories that demonstrate the manner in which the Oersted field influences switching dynamics. For a system with a thick reference layer and no pinning, we apply a large current density $J = 2.5\ 10^{11}$ A/m$^2$ that is linearly ramped up in 65 ps and left on for the remainder of the simulation. This current results in fast reversal, which we examine with and without including the Oersted field from the write channel. In Fig. S5(a) the P→AP transition for Pt devices is seen to become markedly faster under the influence of $H_{Oe}$. The magnetization crosses the hard-axis saddle-point one full oscillation earlier

than it otherwise would. Meanwhile, the AP→P transition remains essentially unchanged in terms of speed. Since it appears that the Oersted field has the greatest impact in the early stages of the dynamics, we run simulations where we turn off the Oersted field after some time $\tau_{Oe}$ less than the duration of the current pulse. For the P→AP transition, we find that $\boldsymbol{H}_{Oe}$ must be left on for approximately 0.25 ns to provide switching assistance akin to that seen in Fig. S5(a), otherwise the dynamics are largely unaffected. This confirms that the Oersted field contributes to the switching primarily through a large initial torque. In Fig. S5(b), we show that reversing the sign of the Oersted field for Pt devices ($\xi_{SH}$=0.08) has a profound impact on the switching dynamics. As mentioned in the main text, the dynamics become notably more complex and there is a substantial delay before AP→P finally occurs. The P→AP transition is completely suppressed under these conditions. In Fig. S5(c) we show that in Ta devices $\boldsymbol{H}_{Oe}$ has comparatively little impact on the dynamics. This is because of the increased $\xi_{SH}$=-0.12 in Ta, which renders $\boldsymbol{H}_{Oe}$ 50% weaker in relative terms. Nevertheless, the P state is slightly delayed, which is the expected result of the Oersted field stymying switching in the P→AP direction. Finally, it is worth noting that switching in Pt devices with $\boldsymbol{H}_{Oe}$ approaches the speed of switching in Ta devices for the same current density — yet another benefit of choosing Pt as the spin Hall channel material.

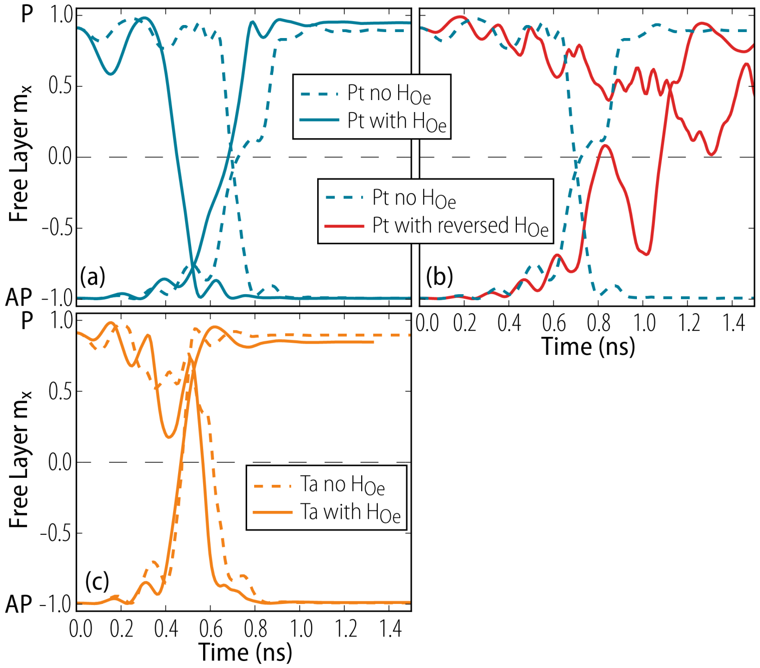


Figure S5: A comparison of reversal trajectories with and without the Oersted field for (a) unpinned Pt devices (b) unpinned Ta devices, (c) unpinned Pt devices with a reversed Oersted field, and (d) a direct comparison of Ta and Pt devices switching trajectories.

# References:


[1] M.-H. Nguyen, D.C. Ralph, and R.A. Buhrman, Phys. Rev. Lett. **116**, 126601 (2016).

[2] M.-H. Nguyen, C.-F. Pai, K.X. Nguyen, D.A. Muller, D.C. Ralph, and R.A. Buhrman, Appl. Phys. Lett. **106**, 222402 (2015).

[3] C.F. Pai, M. Nguyen, C. Belvin, L.H. Vilela-Leão, D.C. Ralph, and R.A. Buhrman, Appl. Phys. Lett. **104**, 082407 (2014).

[4] D. M Pozar, *Microwave Engineering, 3rd Edition* (2005).

[5] M.J. Donahue and D.G. Porter, *OOMMF User's Guide, Version 1.0* (1999).
